# Supplementary material for: Phase field model for viscous inclusions in anisotropic networks
Source: arXiv:2505.06432 source file (2025-07-04)
Supplement: Supplementary file 1 [file Supplement.pdf]

# SUPPLEMENTARY MATERIAL: Phase field model for viscous inclusions in anisotropic networks

Aakanksha Gubbala*[1], Anika M. Jena*[2], Daniel P. Arnold[2], and Sho C. Takatori[1]

[1]Department of Chemical Engineering, Stanford University, Stanford, CA 94305
[2]Department of Chemical Engineering, University of California, Santa Barbara, Santa Barbara, CA 93106

## Contents

**1 Detailed Experimental Methods** **2**
1.1 Buffers . . . 2
1.2 Actin and myosin preparation . . . 2
1.3 Giant unilamellar vesicle (GUV) preparation . . . 2
1.4 Surface preparation . . . 2
1.5 Assembling actin cortex on a lipid bilayer . . . 3
1.6 Microscope for all imaging experiments . . . 3

**2 Image Analysis** **3**
2.1 Classification of Samples . . . 3
2.2 Domain Growth Calculation . . . 3
2.3 Curvature Calculation . . . 4

**3 Phase Field Theory** **4**
3.1 Model Development . . . 4
3.2 Non-dimensionalization . . . 6
3.3 Linear Stability Analysis . . . 6

**4 Numerical Implementation** **7**

**5 Figures** **9**

## Video Captions

**Video S1:** Experimental time-lapse of the domains (green, *left*), actin (red, *center*), and a composite of the two channels (*right*), is presented for low and high actin density (top and bottom row respectively). Scale bar is 5 µm.

**Video S2:** Numerical solutions to the theoretical model for model parameters $(E_1, \phi_o) = (0.1, 0.3)$, (low actin density, *top*) and $(E_1, \phi_o) = (2, 0.75)$, (high actin density, *bottom*). Rest of the model parameters are $(\beta, \gamma, \chi) = (1, 0.1, 1)$ and $E_3 = E_1$. The lengths and time are presented in non-dimensional units.

# 1 Detailed Experimental Methods

## 1.1 Buffers

Filamentous actin buffer (F-buffer) consists of 50 mM Tris (pH 7.5), 2 mM magnesium chloride, 0.5 mM adenosine triphosphate (ATP), 0.2 mM calcium chloride, 25 mM potassium chloride, and 1 mM dithiothreitol (DTT). DTT was added to all buffers immediately before use to preserve its reactivity.

Assay buffer (A-buffer) consists of 25 mM imidazole (pH 7.4), 4 mM magnesium chloride, 1 mM (ethylene glycol-bis(β-aminoethyl ether)-N,N,N',N'-tetraacetic acid) (EGTA), 25 mM potassium chloride, and 1 mM DTT.

Globular actin buffer (G-buffer) consists of 2 mM Tris (pH 8.0), 0.2 mM calcium chloride, 0.5 mM DTT, 1 mM sodium azide, and 0.2 mM ATP.

## 1.2 Actin and myosin preparation

Rabbit skeletal muscle actin was purified from muscle acetone powder (Pel-Freez, catalog no: 41995-2, Lot 16743) using standard methods[1,2]. No rabbits or other animals were directly involved in this study. Actin was stored as depolymerized globular actin (G-actin) at -80°C in G-buffer with 6% sucrose until use.

Actin was labeled with fluorescent Alexa Fluor 555 NHS Ester (Succinimidyl Ester) (Invitrogen catalog no: A20009) for microscopic visualization. G-actin was reacted with NHS-Alexa Fluor 555 in HEPES buffer at room temperature for 30 minutes. 2x-concentrated F-buffer was then added to the G-actin, quenching the NHS reaction and causing G-actin to polymerize to F-actin. F-actin polymerization proceeded for 30 minutes at room temperature, and then overnight at 4°C. Labeled F-actin was centrifuged at 142,000 $\times$ g for 30 minutes, and the pellet collected. Unreacted dye and defective G-actin monomers and oligomers that were unable to polymerize were discarded in the supernatant. Labeled F-actin was dissolved in G-buffer, and allowed to de-polymerize for three days at 4°C before freezing and storing in 6% sucrose at -80°C.

## 1.3 Giant unilamellar vesicle (GUV) preparation

Giant unilamellar vesicles (GUVs) were prepared using the established method of electroformation[3]. Briefly, lipids were mixed with the following composition: 45.7% 1,2-dioleoyl-sn-glycero-3-phosphocholine (DOPC, Avanti catalog no: 850375P), 34.7% 1,2-dipalmitoyl-sn-glycero-3-phosphocholine (DPPC, Avanti catalog no: 850355C), 15% cholesterol (TCI Chemical, catalog no: C3624), 4% 1,2-dioleoyl-3-trimethylammonium-propane (DOTAP, Avanti catalog no: 890890P), 0.3% 1,2-distearoyl-sn-glycero-3-phosphoethanolamine-N-[poly(ethylene glycol)2000-N'-carboxyfluorescein] (DSPE-PEG2k-FITC, Avanti catalog no: 810120C), and 0.3% ATTO 647-labeled 1,2-dioleoyl-sn-glycero-3-phosphoethanolamine (ATTO 647-DOPE, ATTO-TEC catalog no: AD 647-161). Compositional variations were achieved by sampling different vesicles within the diverse population that formed under these conditions. An additional set of vesicles was formed using 52.7% DOPC, 24.7% DPPC, 8% DOTAP, 0.3% DSPE-PEG2k-FITC, and 0.3% ATTO 647-DOPE, to achieve the lowest area fraction sampled amongst the active samples. Lipids were spread on an indium tin oxide (ITO)-coated microscope slide (Diamond Coatings, 8-12 Ohm slide) and dried under vacuum for 30 minutes.

A 2 mm rubber gasket was sandwiched between the ITO-coated slide containing lipids and a clean ITO-coated slide, and the interstitial space filled with 75 mM sucrose solution. A sinusoidal electric potential of amplitude 3V (peak-to-peak) and frequency 10 Hz was applied to the chamber for two hours at 50 °C. After two hours, the frequency was changed to 2 Hz for 30 minutes. The resulting GUVs were collected, stored at room temperature and used within one day.

## 1.4 Surface preparation

Glass cover slips No. 1.5 (Fisher) were cleaned with piranha solution (3:1 sulfuric acid:hydrogen peroxide) for five minutes and then washed with deionized water. The cover slips were then made hydrophobic via reaction with trimethylchlorosilane (Sigma) vapors in a vacuum chamber, under house vacuum for fifteen minutes. A 6 mm cylindrical polydimethylsiloxane (PDMS) chamber was attached to the cover slip surface to hold liquids.

Cover slips were incubated with 200 nM heavy meromyosin (HMM) for five minutes. After five minutes, 0.1 mg/mL polylysine-grafted-PEG (PLL-g-PEG) was added and the HMM/PLL-g-PEG solution incubated for another five minutes. The coverslip was then washed, first with A-buffer, and then with MilliQ water.

### 1.5 Assembling actin cortex on a lipid bilayer

GUVs in MilliQ water were added to the cover slip chamber. The cover slip was heated to 37°C for at least 20 minutes, during which time GUVs ruptured on the treated surface. Unbound GUVs were then washed from the cover slip with A-buffer. F-actin spontaneously adsorbed to the liquid-ordered phase of lipid bilayer via electrostatic attraction to DOTAP[4]. Unbound actin was washed from the cover slip with A-buffer. The actin filaments are 3 to 5 microns long.

### 1.6 Microscope for all imaging experiments

All imaging was carried out on an inverted Nikon Ti2-Eclipse microscope (Nikon Instruments) using an oil-immersion objective (Apo 100x, NA 1.45, oil). Lumencor SpectraX Multi-Line LED Light Source was used for excitation (Lumencor, Inc). Fluorescent light was spectrally filtered with emission filters (432/36, 515/30, 595/31, and 680/42; Semrock, IDEX Health and Science) and imaged on a Photometrics Prime 95 CMOS Camera (Teledyne Photometrics). Microscope images were collected using MicroManager 1.4 software[5].

## 2 Image Analysis

### 2.1 Classification of Samples

Due to the heterogeneity in creating the experimental samples, the extent of growth suppression may vary among different samples. To address this heterogeneity, we classify our samples and calculate an average over them. We choose the actin density metric $\rho$, which estimates the amount of actin in the Ld phase (see Fig. S1).[6] Samples with high actin density have sharper deformations in lipid domains, while low actin density samples remain nearly circular.

From the actin density values in Fig. S1, it is clear that there are 2 low actin density samples and 1 high actin density sample. There are two intermediate densities clustered around $\rho/\rho_{\max} = 0.5$, suggesting a "medium" actin density group. Upon careful analysis of growth kinetics and curvature distribution, we find that the "medium" actin density samples exhibit structural features similar to the low and high actin density groups. Hence, we assume a binary classification of our samples. In Fig. 2 of the main text and Fig. S2, we present an average over 3 low actin density samples and 2 high actin density samples.

### 2.2 Domain Growth Calculation

Low resolution microscope images are first interpolated to create a large matrix of size $2048^2$ to accurately detect the boundaries of the domains in the subsequent analysis. The matrices are then binarized using the Otsu threshold value to transform them into a level-set representation. The average size of domains $R(t)$ is calculated by taking the inverse of the first moment of the static structure factor $S(k,t)$:

$$R(t) = \frac{\int_0^{k_{\text{cut}}} S(k,t)\ dk}{\int_0^{k_{\text{cut}}} kS(k,t)\ dk}\ , \tag{S1}$$

where $k = |\boldsymbol{k}|$ is the radially averaged wave number, and the cut-off wavelength for integration is $k_{\text{cut}} = 50 \times k_{\max}$, where $k_{\max}$ is the wave number corresponding to the peak of $S(k,t)$. The structure factor is defined as $S(k,t) = \langle \phi_{\boldsymbol{k}}(t)\phi_{-\boldsymbol{k}}(t)\rangle$, where $\phi_{\boldsymbol{k}}$ is the Fourier transform of the concentration field $\phi(\boldsymbol{x},t)$. For experiments, we approximate $\phi$ as the level-set representation of the Lo images. We bin the structure factor spectra to remove small fluctuations.

### 2.3 Curvature Calculation

From the level-set representation of an image, the zero-level contour of each identifiable closed-loop domain represents the domain boundary and is extracted using standard tools from the skimage library in Python (see Fig. S3 for more details). The unsigned curvature $\kappa$ is calculated using a parametric representation of the domain boundary $g(u) = (x(u), y(u))$:

$$\kappa = \frac{|x'y'' - y'x''|}{(x' + y')^{3/2}} \ . \tag{S2}$$

Finally, to emphasize the curvature heterogeneity of each domain, $\kappa$ is normalized by its maximum value.

# 3 Phase Field Theory

## 3.1 Model Development

We start with the basic free energy of a phase-separating nematic-isotropic fluid mixture:

$$F[\phi, \boldsymbol{Q}] = F_\phi + \int (f_{\text{bulk}} + f_{\text{elastic}})\ d\boldsymbol{x}\ , \tag{S3}$$

where

$$F_\phi = \int \left( \frac{\phi^4}{4} - \frac{\phi^2}{2} + \frac{1}{2}|\nabla\phi|^2 \right) d\boldsymbol{x} \tag{S4}$$

is the classical Cahn-Hilliard free energy of phase separation [7,8] and

$$f_{\text{bulk}} = \frac{\beta}{4} Q_{ij}Q_{jk}Q_{kl}Q_{li} - \frac{A}{2} Q_{ij}Q_{ij} \tag{S5}$$

is the Landau-de Gennes energy controlling the isotropic-to-nematic phase transition [9]. It takes the form of a double-well potential, where $A$ is typically a function of temperature and $\beta > 0$ always. The saturation value of $Q_{ij}$ is given by the critical points of Eq. S5, which are $\pm\sqrt{A/(2\beta)}$. We let $A = 1 + \phi$, such that the free energy is isotropic for $\phi = -1$ and nematic for $\phi = +1$.

The isotropic-to-nematic transition is more accurately captured by the following free energy expression for lyotropic liquid crystals,

$$f_{\text{bulk}} = -A(\mu)Q_{ij}Q_{ij} + BQ_{ij}Q_{jk}Q_{kl}Q_{li}\ . \tag{S6}$$

One can instead choose concentration as the control parameter and write $A(\phi) = (1 + \phi)/2$. This is a linear approximation where $\mu \sim \phi$ for small concentration fluctuations, characteristic of a smooth mean-field theory. Otherwise, the resulting set of equations becomes a highly nonlinear problem. While the large density jump associated with the isotropic-to-nematic transition is relevant for studying the critical properties of the model, we can neglect this jump because our interest lies in the fully phase-separated phases within the off-critical regimes. Furthermore, the $A(\phi)$ approximation has been used to model lyotropic liquid crystals in prior literature. [10,11]

To construct the double-well potential, we chose powers of $\text{Tr}(\boldsymbol{Q}^2) \equiv Q_{ij}Q_{ij}$ because they are the only independent rotationally invariant term in 2D. In 3D, $\text{Tr}(\boldsymbol{Q}^3) \equiv Q_{ij}Q_{jk}Q_{ki}$ is also rotationally invariant, so it is also included in the Landau-de Gennes free energy to describe the isotropic-to-nematic transition [9]. To verify rotational invariance, we define a rotation matrix $\boldsymbol{R}$, where $\boldsymbol{Q}$ transforms as $\boldsymbol{RQR}^T$ and $\boldsymbol{RR}^T = \boldsymbol{R}^T\boldsymbol{R} = \boldsymbol{I}$. For the quadratic term, the proof of rotational invariance is straightforward, as shown below:

$$(\boldsymbol{RQR}^T)^2 = \boldsymbol{RQR}^T\boldsymbol{RQR}^T = \boldsymbol{RQ^2R}^T \tag{S7}$$

Rotating the $\boldsymbol{Q}$ tensor is equivalent to rotating the $\boldsymbol{Q}^2$ tensor. Other powers of $\boldsymbol{Q}$ depend on $\text{Tr}(\boldsymbol{Q}^2)$ and $\text{Tr}(\boldsymbol{Q}^3)$ due to the Cayley-Hamilton theorem, which states that for a square matrix, $\boldsymbol{Q}$ satisfies:

$$\boldsymbol{Q}^3 - \text{Tr}(\boldsymbol{Q})\boldsymbol{Q}^2 + \frac{1}{2}(\text{Tr}(\boldsymbol{Q})^2 - \text{Tr}(\boldsymbol{Q}^2))\boldsymbol{Q} - (\det \boldsymbol{Q})\boldsymbol{I} = 0 \tag{S8}$$

which simplifies to $\boldsymbol{Q}^3 = \frac{1}{2}\mathrm{Tr}(\boldsymbol{Q}^2)\boldsymbol{Q} + (\det \boldsymbol{Q})\boldsymbol{I}$ due to the traceless property of the $\boldsymbol{Q}$ tensor. In 2D, since $\det \boldsymbol{Q} = -\frac{1}{2}\mathrm{Tr}(\boldsymbol{Q}^2)$, we can express $\boldsymbol{Q}^3$ a function of $\boldsymbol{Q}^2$. Thus, the quadratic term $\mathrm{Tr}(\boldsymbol{Q}^2)$ is the only independent rotational invariant quantity.

The simplest elastic energy of a nematic is given by

$$f_{\text{elastic}} = \frac{1}{2}E_1 \partial_i Q_{jk} \partial_i Q_{jk} \ , \tag{S9}$$

where $E_1$ is the Frank elastic constant. For convenience, we use the derivative shorthand $\partial_i \equiv \partial/\partial x_i$ in this document.

Assuming conserved dynamics for $\phi$ and non-conserved dynamics for $Q_{ij}$, the evolution equations are given by

$$\frac{\partial \phi}{\partial t} = \gamma \nabla^2 \frac{\delta F}{\delta \phi}, \quad \frac{\partial \mathbf{Q}}{\partial t} = -\frac{\delta F}{\delta \mathbf{Q}} \ . \tag{S10}$$

Eqs. S3-S10 describe the phase separation dynamics of a nematic and an isotropic fluid. The quadratic gradient energy in Eq. S9 favors uniaxial ordering, resulting in the formation of stripes of nematic and isotropic phase at long times. While the terms "uniaxial" and "biaxial" are sometimes used to indicate the optical axes in liquid crystals, we instead use these terms to refer to the alignment of the nematic fields. We use the term "uniaxial" to describe the alignment of the nematic phase into straight lines due to the quadratic elastic energy terms, which favor the orientation of rods in a single direction. Through the term "biaxial", we intend to convey the splay and bend phenomena that result in unusual domain structures. One way to quantify the deviation from uniaxial behavior is to examine the topological defects or analogously, curvature distributions. As shown in Fig. 4 of the main text, large variations in curvature are characteristic of sharply cusped structures.

To promote the formation of triangular structures, we consider two non-linear effects: anchoring and elastic anisotropy. We experimentally observe that actin filaments conform to the shape of the droplet, creating cusps where the filaments are splayed. To orient the nematic field along the domain interface, we define the free energy density of anchoring as:

$$f_{\text{anch}} = \frac{1}{2}\chi(\boldsymbol{n} \cdot \nabla\phi)^2 \ , \tag{S11}$$

where $\chi$ is the coefficient of anchoring. If the nematic director $\boldsymbol{n}$ is aligned with the interface normal $\nabla\phi$, then the anchoring energy is zero. We can write Eq. S11 as

$$f_{\text{anch}} = \frac{1}{2}\chi(n_i n_j \partial_i \phi \partial_j \phi) \ . \tag{S12}$$

We substitute the definition of the nematic tensor field, $Q_{ij} = S(n_i n_j - \delta_{ij}/2)$ in the above equation to give

$$f_{\text{anch}} = \frac{1}{2}\chi\left(\frac{1}{S}Q_{ij}\partial_i\phi\partial_j\phi + \frac{1}{2}|\nabla\phi|^2\right) \ , \tag{S13}$$

which is Eq. 7 of the main text. The second term is combined with the gradient energy in Eq. S4 to give an effective line tension parameter, $\lambda = 1 + \chi/2$.

In Fig. S4, we find that the nematic field still enforces uniaxial ordering, but the inclusion of anchoring conforms the field around the isotropic droplet, producing tactoid shapes. To break uniaxial order, which is favored by quadratic terms in 2D, we need to introduce a higher order elastic gradient energy for the nematic. So, Eq. S9 is modified to

$$f_{\text{elastic}} = \frac{1}{2}E_1 \partial_i Q_{jk} \partial_i Q_{jk} + \frac{1}{2}E_3 Q_{ij} \partial_i Q_{kl} \partial_j Q_{kl} \ . \tag{S14}$$

The second term is a widely used form of cubic gradient energy, although other formulations exist that respect rotational invariance[9,12]. In Fig. S4, we find that the addition of elastic anisotropy produces biaxial effects, creating elongated domains.

There exists another quadratic energy term of the type $\partial_i Q_{ik} \partial_j Q_{jk}$. The functional derivative of $\partial_i Q_{ik} \partial_j Q_{jk}$ is

$$A_{ij} = \frac{\delta}{\delta Q_{ij}}(\partial_m Q_{mk} \partial_n Q_{nk}) = 2\partial_j \partial_k Q_{ik} = 2\begin{pmatrix} \partial_x^2 Q_{xx} + \partial_x\partial_y Q_{xy} & \partial_y^2 Q_{xy} + \partial_x\partial_y Q_{xx} \\ \partial_x^2 Q_{xy} - \partial_x\partial_y Q_{yy} & -\partial_y^2 Q_{xx} + \partial_x\partial_y Q_{xy} \end{pmatrix} \tag{S15}$$

which is neither symmetric ($A_{ij} \neq A_{ji}$) nor traceless ($A_{ii} \neq 0$), violating the intrinsic properties of the $Q_{ij}$ tensor. To make Eq. S15 symmetric and traceless, we use the following transformation:

$$A_{ij}^{st} = \frac{1}{2}\left(A_{ij} + A_{ji} - A_{kk}\delta_{ij}\right) = \begin{pmatrix} \nabla^2 Q_{xx} & \nabla^2 Q_{xy} \\ \nabla^2 Q_{xy} & -\nabla^2 Q_{xx} \end{pmatrix} = \nabla^2 Q_{ij} \tag{S16}$$

Both quadratic energy terms have the same functional derivative, and thus exhibit the same dynamical behavior. In 3D, the difference between the two manifests as out-of-plane twists (through terms like $\partial_x\partial_z Q_{ij}, \partial_y\partial_z Q_{ij}$). For this reason, we chose a cubic gradient energy to introduce anisotropic effects.

### 3.2 Non-dimensionalization

In dimensional form, the evolution equations are

$$\frac{\partial\phi}{\partial\bar{t}} = M\bar{\nabla}^2\left(\phi^3 - \phi - \frac{1}{2}Q_{ij}Q_{ij} - \frac{1}{S}\bar{\partial}_j(\alpha Q_{ij}\bar{\partial}_i\phi) - \left(\tilde{\lambda} + \frac{\alpha}{2}\right)\bar{\nabla}^2\phi\right) \tag{S17}$$

$$\begin{aligned}\frac{1}{\Gamma}\frac{\partial Q_{ij}}{\partial\bar{t}} &= [1 + \phi - \beta\, Q_{kl}Q_{kl}]Q_{ij} - \frac{\alpha}{2S}\left(\bar{\partial}_i\phi\,\bar{\partial}_j\phi - \frac{1}{2}\delta_{ij}|\bar{\nabla}\phi|^2\right) + L_1\,\bar{\nabla}^2 Q_{ij} \\ &+ \frac{1}{2}L_3\left(\bar{\partial}_i Q_{kl}\,\bar{\partial}_j Q_{kl} - 2\,\bar{\partial}_k Q_{ij}\,\bar{\partial}_l Q_{kl} - 2\,Q_{kl}\,\bar{\partial}_k\bar{\partial}_l Q_{ij} - \frac{1}{2}\delta_{ij}(\bar{\partial}_k Q_{jl})^2\right)\,,\end{aligned} \tag{S18}$$

where $\phi$ and $Q_{ij}$ are the dimension-less concentration and nematic fields respectively, $M$ is the lipid mobility, $\alpha$ is the coupling parameter, and $\tilde{\lambda}$ is the surface tension parameter. The nematic relaxation time is given by $t_Q = \Gamma^{-1}$, $L_1$ is the Frank elastic constant, and $L_3$ is an elastic constant representing the cubic anisotropy.

We define $l_c = \sqrt{\tilde{\lambda}}$ as the characteristic length of our system, corresponding to the width of the Lo-Ld interface. The characteristic time scale is defined as $t_c = \Gamma^{-1}$, which describes the 'rotational viscosity' of the nematic phase. After defining the non-dimensional variables $\nabla = l_c\bar{\nabla}$ and $t = \bar{t}/t_c$, we are left with 5 dimensional numbers: $E_1 = L_1/l_c^2$, $E_3 = L_3/l_c^2$, and $\chi = \alpha/l_c^2$. The non-dimensional surface tension parameter is $\lambda = \tilde{\lambda} + \chi/2$. The ratio of the two characteristic timescales is given by $\gamma = M/(\tilde{\lambda}\Gamma) = t_Q/t_\phi$. Here, $t_\phi = \tilde{\lambda}/M$ is the timescale of diffusion of $\phi$ across the interface.

### 3.3 Linear Stability Analysis

The evolution equations are

$$\frac{\partial\phi}{\partial t} = \gamma\nabla^2\left[\phi^3 - \phi - \frac{1}{2}Q_{ij}Q_{ij} - \lambda\nabla^2\phi - \frac{\chi}{S}\partial_j(Q_{ij}\partial_i\phi)\right], \tag{S19}$$

$$\begin{aligned}\frac{\partial Q_{ij}}{\partial t} &= [1 + \phi - \beta\, Q_{kl}Q_{kl}]Q_{ij} - \frac{\chi}{2S}\left(\partial_i\phi\,\partial_j\phi - \frac{1}{2}\delta_{ij}|\nabla\phi|^2\right) + E_1\,\nabla^2 Q_{ij} \\ &+ \frac{1}{2}E_3\left(\partial_i Q_{kl}\,\partial_j Q_{kl} - 2\,\partial_k Q_{ij}\,\partial_l Q_{kl} - 2\,Q_{kl}\,\partial_k\partial_l Q_{ij} - \frac{1}{2}\delta_{ij}(\partial_k Q_{jl})^2\right)\,,\end{aligned} \tag{S20}$$

We define the base state as the nematic phase $\phi = +1$ and the director is parallel to the x-axis, giving $Q_{xx} = S$ and $Q_{xy} = 0$. We choose $S = 1/\sqrt{\beta}$ to satisfy the non-linear bulk free energy in Eq. S20. To each field, we add the following perturbations:

$$\phi = 1 + \tilde{\phi}(t)e^{ik_jx_j}\,, \tag{S21}$$

$$Q_{xx} = 1/\sqrt{\beta} + \tilde{Q}_{xx}(t)e^{ik_jx_j}\,, \tag{S22}$$

$$Q_{xy} = \tilde{Q}_{xy}(t)e^{ik_jx_j}\,. \tag{S23}$$

Substituting the above expressions in Eqs. S19-S20 gives

$$\frac{d\tilde{\phi}}{dt} = -\gamma k^2 \left[2 + \lambda k^2 + \chi(k_x^2 - k_y^2)\right] \tilde{\phi} + \frac{4\gamma}{\sqrt{\beta}} k^2 \tilde{Q}_{xx} = -\omega_\phi \tilde{\phi} - \omega_{12} \tilde{Q}_{xx} \ , \tag{S24}$$

$$\frac{d\tilde{Q}_{xx}}{dt} = -\left[4 + E_1 k^2 + \frac{E_3}{\sqrt{\beta}}(k_x^2 - k_y^2)\right] \tilde{Q}_{xx} + \frac{1}{\sqrt{\beta}} \tilde{\phi} = -\omega_{xx} \tilde{Q}_{xx} - \omega_{21} \tilde{\phi} \ , \tag{S25}$$

$$\frac{d\tilde{Q}_{xy}}{dt} = -E_1 k^2 \tilde{Q}_{xy} = -\omega_{xy} \tilde{Q}_{xy} \ , \tag{S26}$$

where $\omega_i$ denotes the growth rate of fluctuations. From Eq. S24-Eq. S25, we find that initial perturbations to the horizontal nematic phase result in different fluctuations in the $x$ and $y$ directions. The growth rates of these fluctuations, $\omega_i$, are controlled by the parameters $\chi, \lambda, E_1, E_3, \beta$. We know by definition that $E_1 > 0$, $\gamma > 0$, and $\beta > 0$. Thus, the growth rates $\omega_{12}$, $\omega_{21}$, and $\omega_{xy}$ are strictly positive. The expanded forms of $\omega_\phi$ and $\omega_{xx}$ are

$$\omega_\phi = \gamma k^2 \left[2 + \left(1 + \frac{3}{2}\chi\right) k_x^2 + \left(1 - \frac{\chi}{2}\right) k_y^2\right] \geq 0 \ , \tag{S27}$$

$$\omega_{xx} = 4 + \left(E_1 + \frac{E_3}{\sqrt{\beta}}\right) k_x^2 + \left(E_1 - \frac{E_3}{\sqrt{\beta}}\right) k_y^2 \geq 0 \ . \tag{S28}$$

For the above expressions to be positive, we need to have $-2/3 \leq \chi \leq 2$ and $\beta \geq (E_3/E_1)^2$.

# 4 Numerical Implementation

Consider a square lattice of size $N^2$ where $N = 512$ and length $L = 500$. To solve Eqs. S19-S20, we use pseudospectral methods with a Fourier basis, which naturally imposes periodicity in all directions. Let the subscript $\boldsymbol{k}$ denote the Fourier-transformed function, where the vector components $(k_x, k_y) = (2\pi m/L, 2\pi n/L)$; $m, n \in \left\{-\frac{N}{2}, -\frac{N}{2}+1, \cdots, \frac{N}{2}-1\right\}$ represent the spatial frequencies. The resulting equations are

$$\frac{d\phi_{\boldsymbol{k}}}{dt} = -\gamma k^2 \Big( \left\{\phi^2 - \phi - \frac{1}{2} Q_{ij} Q_{ij} - \chi \partial_j (Q_{ij} \partial_i \phi)\right\}_{\boldsymbol{k}} + \kappa k^2 \phi_{\boldsymbol{k}} \Big) + k^6 \phi_{\boldsymbol{k}} - k^6 \phi_{\boldsymbol{k}} \ , \tag{S29}$$

$$\frac{d(Q_{ij})_{\boldsymbol{k}}}{dt} = \left\{[1 + \phi - \beta Q_{kl} Q_{kl}] Q_{ij} - \frac{1}{2}\chi \left(\partial_i \phi \partial_j \phi - \frac{1}{d}\delta_{ij} |\nabla \phi|^2\right)\right\}_{\boldsymbol{k}} - E_1 k^2 (Q_{ij})_{\boldsymbol{k}} + E_3 \{\cdot\}_{\boldsymbol{k}} \ . \tag{S30}$$

where $k = |\boldsymbol{k}|$. The notation $\{\cdot\}$ serves as a shorthand for the long expressions for that term (see Eqs. S19-S20 for the complete expression). We add and subtract a large dampening term, $\nabla^6 \phi \to -k^6 \phi_{\boldsymbol{k}}$ for numerical stability[13]. To discretize the equations, we implement the IMEX (IMplicit-EXplicit) scheme. All linear terms are treated implicitly, with the exception of the dampening terms, where only one of the terms is implicit. We also apply a de-aliasing filter (remove 1/3 of largest modes) to the non-linear terms for accuracy[14]. After applying the forward Euler discretization for a time step $\Delta t$, we get the following equations:

$$\phi_{\boldsymbol{k}}^{n+1} = \frac{\phi_{\boldsymbol{k}}^n (1 + k^6 \Delta t) - \gamma k^2 \Delta t \left\{\phi^2 - \phi - \frac{1}{2} Q_{ij} Q_{ij} - \chi \{\cdot\}\right\}_{\boldsymbol{k}}^n}{1 + (\gamma \kappa k^4 + k^6) \Delta t} \ , \tag{S31}$$

$$(Q_{ij})_{\boldsymbol{k}}^{n+1} = \frac{(Q_{ij})_{\boldsymbol{k}}^n + \Delta t \left\{[1 + \phi - \beta Q_{kl} Q_{kl}] Q_{ij} - \frac{\chi}{2}\{\cdot\} + E_3 \{\cdot\}\right\}_{\boldsymbol{k}}^n}{1 + E_1 k^2 \Delta t} \ . \tag{S32}$$

Due to the symmetric and traceless properties of $\mathbf{Q}$, we have only two tensor components, $Q_{xx}$ and $Q_{xy}$. Eqs. S31 and S32 are solved in Python using in-built FFT routines and we use the CUDA library to leverage GPU acceleration. The time step $\Delta t$ is updated using an adaptive algorithm, in which the new time step is calculated as $\Delta t_{\text{new}} = (\tau/\Delta)^{1/5}$, where $\Delta = (\Delta\phi \cdot \Delta Q_{xx} \cdot \Delta Q_{xy})^{1/3}$ is the geometric mean of the variations of the fields. The variations are given by $\Delta X = |X(t; \Delta t_{\text{old}}) - X(t; \Delta t_{\text{old}}/2)|$. Here, $X(t; \Delta t)$ refers to calculating $X(t)$ using a time step $\Delta t$ and $\tau$ is the tolerance for numerical error. In our simulations, $\tau = 10^{-6}$.

The nematic fields $Q_{xx}$ and $Q_{xy}$ are initialized as Gaussian noise with zero mean and a small variance of $10^{-4}$ to trigger the isotropic-nematic phase transitions. The concentration field $\phi$ is similarly initialized as $\phi(\boldsymbol{x}, t = 0) = \phi_o + e(\boldsymbol{x})$, where $e \sim \mathcal{N}(\mu = 0, \sigma^2 = 10^{-4})$, where $\phi_o$ is the average value of the field $\phi$. The simulation code is available at `https://github.com/aakanksha-gubbala/ActinNematics`

We can show that the simulations are self-similar through the normalized structure factor $S(k, t)$, given by

$$S(k,t) = \frac{\langle \phi_{\boldsymbol{k}}(t)\phi_{-\boldsymbol{k}}(t)\rangle}{N^2(\langle \phi^2(\boldsymbol{x},t)\rangle - \langle \phi \rangle^2)} , \tag{S33}$$

where $k$ is the radially-averaged wavenumber, $\phi_{\boldsymbol{k}}(t)$ is the spatial Fourier-transform of $\phi(\boldsymbol{x}, t)$, and $\langle \cdot \rangle$ denotes a spatial average[15,16]. The self-similarity hypothesis states that the evolving structure should be time-independent when scaled by an appropriate length-scale. In 2D, we can define a length- and time- independent quantity $\mathcal{F}(k/k_m(t))$ such that

$$\mathcal{F}(k/k_m(t)) = k_m^2 S(k,t), \;\; k_m(t) = \frac{\sum kS(k,t)}{\sum S(k,t)} . \tag{S34}$$

In Fig. S6, we plot $\mathcal{F}(k/k_m(t))$ as a function of $k/k_m$ and find that we get a master curve, which indicates self-similarity.

# References


[1] J. A. Spudich and S. Watt, *Journal of Biological Chemistry*, 1971, **246**, 4866–4871.

[2] S. MacLean-Fletcher and T. D. Pollard, *Biochemical and Biophysical Research Communications*, 1980, **96**, 18–27.

[3] M. I. Angelova and D. S. Dimitrov, *Faraday Discussions of the Chemical Society*, 1986, **81**, 303.

[4] C. F. E. Schroer, L. Baldauf, L. van Buren, T. A. Wassenaar, M. N. Melo, G. H. Koenderink and S. J. Marrink, *Proceedings of the National Academy of Sciences*, 2020, **117**, 5861–5872.

[5] A. D. Edelstein, M. A. Tsuchida, N. Amodaj, H. Pinkard, R. D. Vale and N. Stuurman, *Journal of Biological Methods*, 2014, **1**, e10.

[6] D. P. Arnold and S. C. Takatori, *Langmuir*, 2024, **40**, 26570–26578.

[7] J. W. Cahn and J. E. Hilliard, *The Journal of Chemical Physics*, 1958, **28**, 258–267.

[8] J. W. Cahn, *Acta Metallurgica*, 1961, **9**, 795–801.

[9] P. G. de Gennes and J. Prost, *The Physics of Liquid Crystals*, Clarendon Press, 1993.

[10] M. L. Blow, S. P. Thampi and J. M. Yeomans, *Physical Review Letters*, 2014, **113**, 248303.

[11] F. Caballero and M. C. Marchetti, *Physical Review Letters*, 2022, **129**, 268002.

[12] C. D. Schimming and J. Viñals, *Soft Matter*, 2022, **18**, 8024–8033.

[13] L. Duchemin and J. Eggers, *Journal of Computational Physics*, 2014, **263**, 37–52.

[14] J. P. Boyd, *Chebyshev and Fourier Spectral Methods: Second Revised Edition*, Courier Corporation, 2001.

[15] J. Zhu, L.-Q. Chen, J. Shen and V. Tikare, *Physical Review E*, 1999, **60**, 3564–3572.

[16] A. J. Bray and A. D. Rutenberg, *Physical Review E*, 1994, **49**, R27–R30.

## 5 Figures

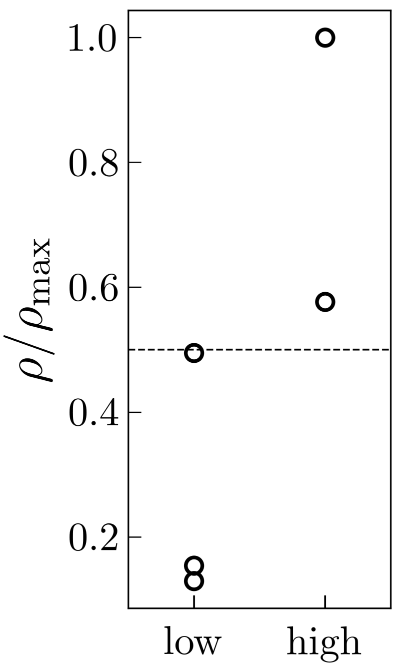


**Figure S1** Actin density $\rho$ is presented for 5 experimental samples. We assume a binary classification of the samples (at a cut-off $\rho/\rho_{\mathsf{max}} = 0.5$, black dotted line), categorizing them into "low" and "high" actin density groups. Actin density is calculated by dividing the mean fluorescence intensity of actin by the available area of the Ld phase. Density is normalized by the maximum value observed, $\rho_{\rm max}$.

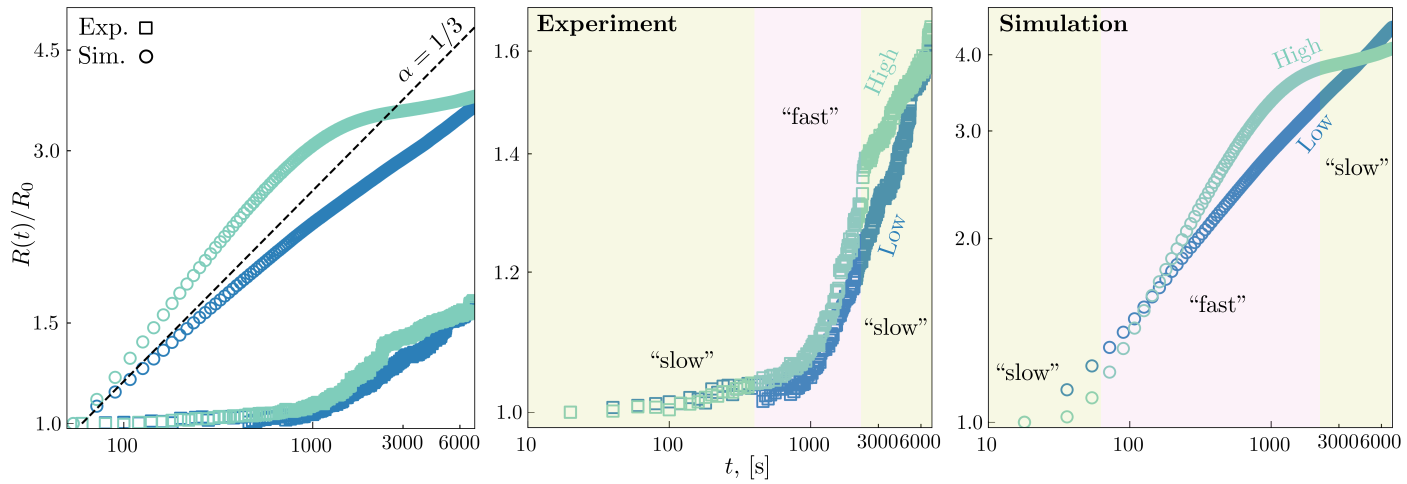


**Figure S2** Average size of Lo domains $R(t)$ is plotted against time $t$. In both experiments (squares) and simulations (circles), we observe 3 growth regimes – slow growth, followed by rapid coarsening, and then reverting to slow linear coarsening at later times.

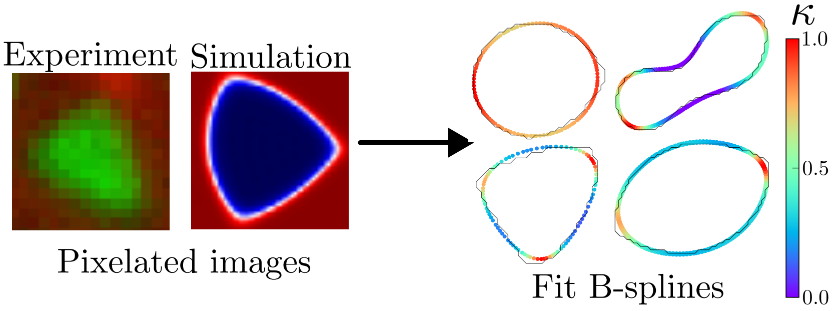


**Figure S3** Each domain boundary is fitted to a B-spline to smooth the jagged features. The spline function is then used to calculate the curvature using Eq. S2. The spatial variation in normalized curvature $\kappa$ is presented as a heat map.

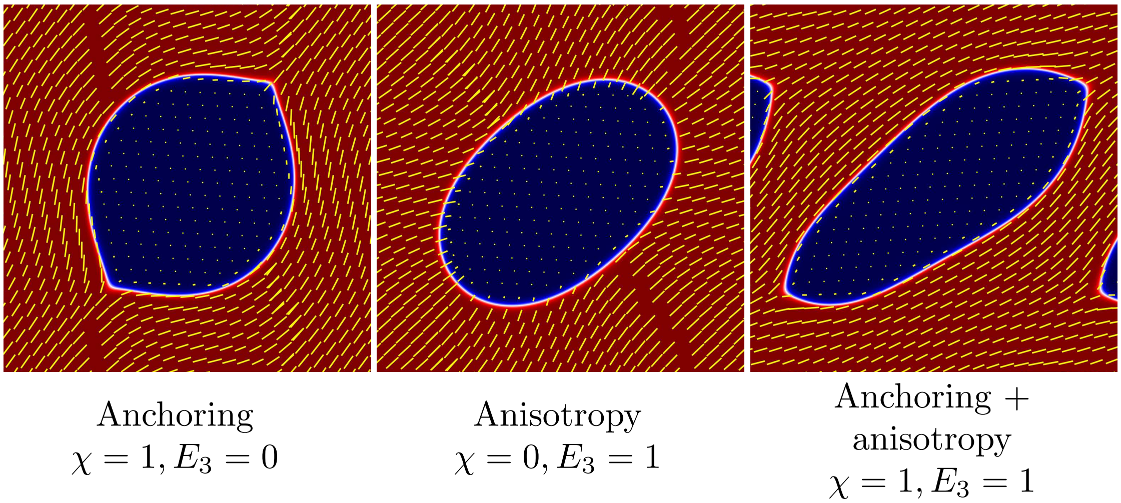


**Figure S4** Simulation snapshots of an isotropic droplet (blue) in a nematic fluid (red) produced by pure nematic anchoring (*left*, $\chi = 1, E_3 = 0$), elastic anisotropy (*center*, $\chi = 0, E_3 = 1$), and a combination of the two effects (*right*, $\chi = E_3 = 1$). Images are cropped to highlight droplet structure. Model parameters used here are: $(\phi_o, \beta, \gamma, E_1) = (0.3, 1, 1, 1)$.

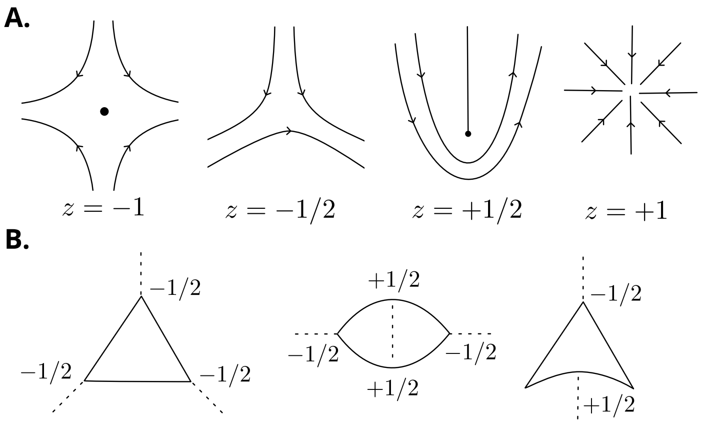


**Figure S5** (A) Schematic of topological defects for charges $z = -1, -1/2, +1/2, +1$. (B) Defect structures may be arranged to produce triangles (*left & right*) and tactoids (*center*).

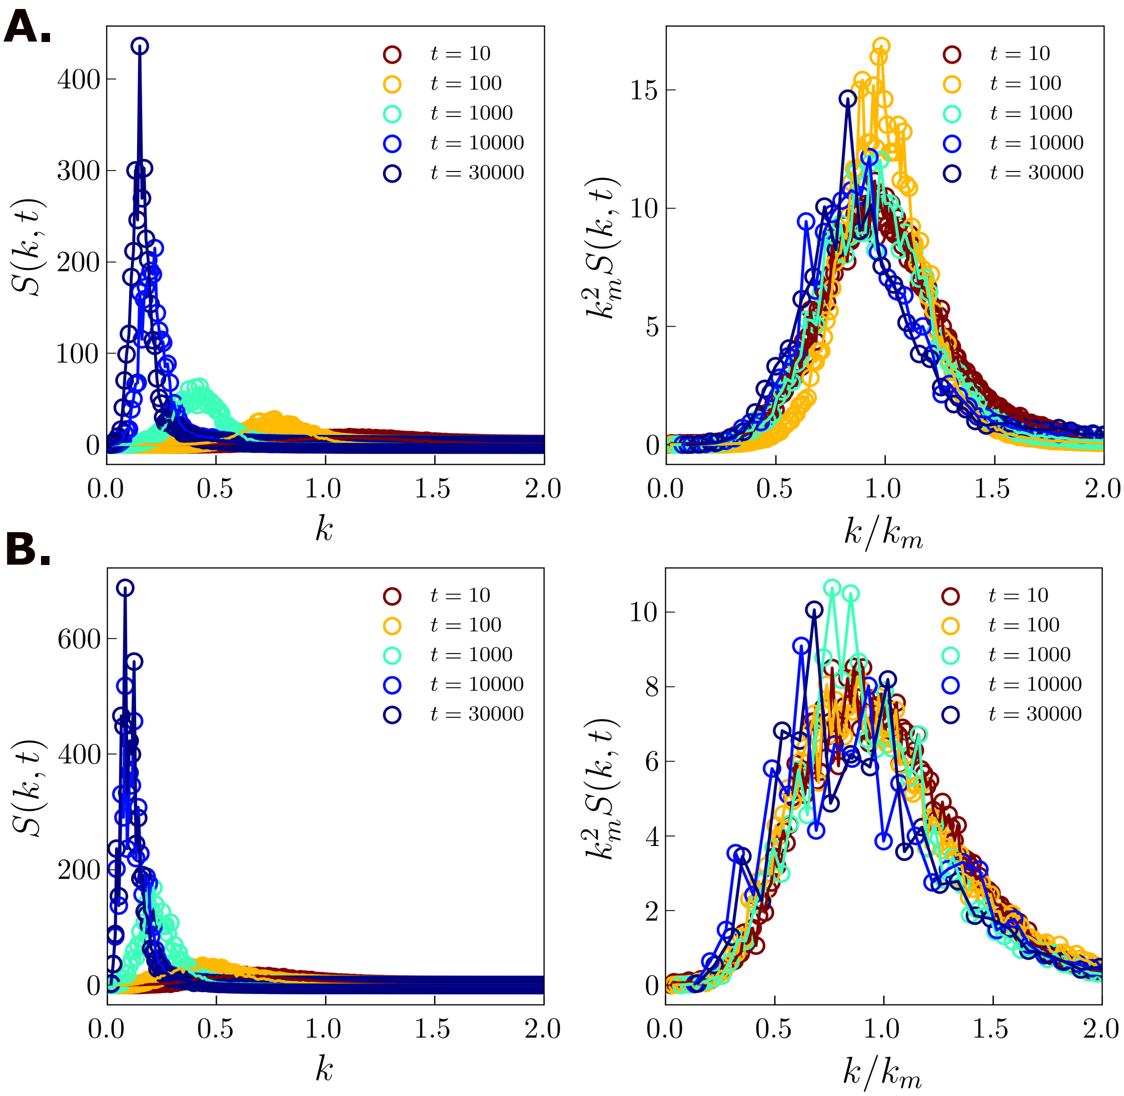


**Figure S6** The self-similarity hypothesis is verified for (A) low ($E_1 = 0.1, \phi_o = 0.3$) and (B) high ($E_1 = 2, \phi_o = 0.75$) actin density simulations. *Left*: Normalized structure factor $S(k,t)$ is plotted as a function of wavenumber $k$. *Right*: The length-independent quantity $k_m^2 S(k,t)$ is plotted as a function of normalized wavenumber $k/k_m$, where $k_m$ is the first moment of $S(k,t)$. Simulation time $t$ has arbitrary units.
